# Supplementary material for: Sparse Binary Transformers for Multivariate Time Series Modeling
Source: arXiv:2308.04637 source file (2023-08-09)
Supplement: Supplementary file 1 [file arch.tex]

Both our Dense and  \gls{sbt} models are developed using PyTorch.  We develop custom multihead attention modules for both the step-t and fixed $\mathbf{Q}, \mathbf{K}, \mathbf{V}$ masks, using the quantized multihead attention module.  We chose this module in order for the masks to be easily extended into other quantization frameworks.  

For step-t attention, we pass a static mask to the attention module. For a model with window size $w=5$, the step-t looks like the following:

\[

  \begin{bmatrix}
    0 & -inf & -inf & -inf & -inf \\
    -inf & 0 & -inf & -inf & -inf \\
    -inf & -inf & 0 & -inf & -inf \\
    -inf & -inf & -inf & 0 & -inf \\
    0 & 0 & 0 & 0 & -inf \\
  \end{bmatrix}
\]

We can extend this to two step forecasting by using the following mask: 

\[

  \begin{bmatrix}
    0 & -inf & -inf & -inf & -inf \\
    -inf & 0 & -inf & -inf & -inf \\
    -inf & -inf & 0 & -inf & -inf \\
    0 & 0 & 0 & -inf & -inf \\
    0 & 0 & 0 & -inf & -inf \\
  \end{bmatrix}
\]

For the fixed $\mathbf{Q}, \mathbf{K}, \mathbf{V}$ mask, we apply a different random fixed mask over each projection.  During model initialization, we create a mask of ones of size (embed dim, window size), and set random indices of size (embed dim*window size*prune rate) equal to zero.  $\mathbf{Q}, \mathbf{K}, and \mathbf{V}$ masks are all randomly initialized independently.

%\textbf{Architecure Details} Each model in our framework consists of 2 encoder layers each with a multi-head attention containing two heads.  The feedforward dimensionality for each model is 256 with ReLU is used for nonlinearity.  Anomaly detection and forecasting rely on a single decoder linear layer which reconstructs the output to size ($m$, $w$), while classification outputs size ($d$, $num. classes$) and takes the mean of $d$ to formulate a final classification prediction.  

\newpage
