# Supplementary material for: Sparse Binary Transformers for Multivariate Time Series Modeling
Source: arXiv:2308.04637 source file (2023-08-09)
Supplement: Supplementary file 2 [file complexity.tex]

We summarize the FLOPs of both the liner layers and multihead attention layers in Table 
\ref{flops_details}.  For classification layers, where we use a 50\% prune rate, both layers generally get a 50\% reduction in the number of FLOPs.  For anomaly detection and forecasting tasks, the models have a more significant reduction in FLOPs due to the step-t mask.  

\begin{table*}[h]
\begin{center}
\setlength{\tabcolsep}{0.27em}
{%
\begin{tabular}{    c|cccc|cc|ccc} 
\toprule
\multicolumn{1}{c}{}&\multicolumn{4}{c}{}&\multicolumn{2}{c}{Dense Transformer}&\multicolumn{3}{c}{Sparse Binary Transformer}\\
%\midrule
\multicolumn{1}{c}{Type}&\multicolumn{1}{c}{Dataset}&$m$&$w$&\multicolumn{1}{c}{$d$}  & Linear & \multicolumn{1}{c}{ Attention}&$p$& Linear &  Attention\\
\hline

 \parbox[t]{2mm}{\multirow{5}{*}{\rotatebox[origin=c]{90}{\footnotesize{Classification}}}}&Heartbeat	&	61	&	405	&	64	&	1,658,880	&	21,349,170	&	0.50	&	8,192	&	8,266,066	\\
&Ins.Wingbeats	&	200	&	30	&	256	&	65,536	&	475,680	&	0.50	&32,768		&	206,880	\\
&Arabic Digits	&	13	&	93	&	64	&	 16,384	&	553,410	&	0.50	&	8,192	&	221,666	\\
&JapaneseVowels	&	12	&	29	&	32	&	8,192	&	 56,434	&	0.50	&	4,096	&	24,194	\\
&FaceDetection	&	144	&	62	&	128	&	32,768	&	999,688	&	0.50	&	16,384	&	404,488	\\
\hdashline
 \parbox[t]{7.2mm}{\multirow{3}{*}{\rotatebox[origin=c]{90}{\footnotesize{\thead{Anomaly\\Detection}}}}}&MSL&	55	&	50	&	110	&	28,160	&	560,500	&	0.75	&	7,040	&	16,380	\\
&SMAP	&	25	&	50	&	50	&	12,800	&	257,500	&	0.75	&	3,200	&	7,500	\\
&SMD	&	38	&	200	&	76	&	19,456	&	6,175,200	&	0.75	&	4,864	&	45,848	\\
\hdashline
 \parbox[t]{2mm}{\multirow{3}{*}{\rotatebox[origin=c]{90}{\footnotesize{Forecast.}}}}&ECL	&	321	&	200	&	350	&	89,600	&	28,150,000	&	0.75	&	22,400	&	209,700	\\
&Weather	&	7	&	200	&	100	&	25,600	&	8,100,000	&	0.50	&	12,800	&	60,200	\\
&ETTm1	&	12	&	200	&	64	&	16,384	&	5,212,800	&	0.50	&	8,192	&	 38,672	\\
\hline
\end{tabular}
\caption{Computational Savings for Linear and Multihead attention layers }\label{flops_details}
 \vspace{-25pt}
\end{center}
\end{table*}
